# Supplementary material for: An Introduction to Probabilistic Spiking Neural Networks: Probabilistic Models, Learning Rules, and Applications
Source: arXiv:1910.01059 source file (2019-11-27)
Supplement: Supplementary file 1 [file appendix_ex.tex]

\section*{Appendix: Additional Details on the ``Examples'' section}
\label{sec:app_ex}

\subsection*{Batch Learning}

For the batch learning example, the training data set is generated by selecting $500$ images of digit ``$1$'' and ``$7$'' from the USPS handwritten digit data set\cite{hull1994usps}. The test set is similarly obtained by using $125$ examples from the USPS data set. We adopt a two-layer SNN, the first layer encoding the input with $256$ input neurons and the second the output with $2$ output neurons. No hidden neurons exist, thus training is done with the batch SGD rule in \eqref{eq:fully-ml-sgd-batch} for $5000$ epochs with constant learning rate $\eta = 0.05$. The model parameters are randomly initialized with uniform distribution in range $[-1,1]$. We assume the $K_a = K_b = 8$ raised cosine basis functions in Fig.~\ref{fig:ex_basis} with the maximum filter duration $\tau = T$. As a baseline, a conventional ANN with the same topology and a soft-max output layer is trained for the same epochs with the same learning rate. The average performance is evaluated based on $10$ trials with different random seeds. 

\vspace{-0.5cm}
\subsection*{online Learning}

In the online prediction task, the sequence $\{a_l\}$ is generated from two sequences with duration $T_s = 25$, one from class $1$ and the other from class $6$, of the SwedishLeaf data set of the UCR archive\cite{UCRArchive2018}, which are normalized within the range $[0,1]$. At every $T_s = 25$ time steps, with probability $0.7$, an all-zero sequence is selected, and otherwise, one of the two mentioned sequences is selected with equal probability. 

In this task, we adopt a fully connected SNN topology that includes $N_\textH$ hidden neurons. In all cases, the SNN contains $K_a = K_b$ weights per synapses, and neurons in which the synaptic and feedback kernels are parameterized using the raised cosine functions in Fig.~\ref{fig:ex_basis}, whose equation can be found in \cite{pillow08:spatio}. We use $K_a = K_b = 5$ basis functions with filter duration $\tau = [0.5 \Delta T, \Delta T, 3 \Delta T, 5 \Delta T, 10 \Delta T]$. When training, the model parameters are randomly initialized as $\set{N}(0, 0.01)$. We use constant learning rates $\eta = 0.01$ for updating the model parameters; $\kappa = 0.5$ for computing the eligibility traces; and baseline control variates of learning signal with moving average constant $0.01$. 

In all experiments, the SNN is trained using Algorithm~\ref{alg:latent-ml-vl} with the addition of a sparsity regularization term. This is obtained by assuming an i.i.d. reference Bernoulli distribution with a desired spiking rate $r \in [0,1]$, i.e., $\log r(\bmh_{\leq T}) = \sum_{t=0}^T \sum_{i \in \set{H}} h_{i,t} \log r + (1 - h_{i,t}) \log (1-r)$. By adding the regularization term $- \alpha \cdot \text{KL}( q_{\bmtheta^\textH}(\bmh_{\leq T} | \bmx_{\leq T}) \parallel r(\bmh_{\leq T}))$ to the ELBO in \eqref{eq:elbo-general}, we have the regularized learning signal as 
\begin{align*}
\tilde{\ell}(\bmx_{\leq T}, \bmh_{\leq T}) = \sum_{t=0}^T \sum_{i \in \set{X}} \log p(x_{i,t} | u_{i,t}) - \alpha \bigg( \sum_{t=0}^T \sum_{i \in \set{H}} h_{i,t} \log \frac{\sigma(u_{i,t})}{r} + (1-h_{i,t}) \log \frac{1- \sigma(u_{i,t})}{1-r} \bigg).
\end{align*}
As a result, the global feedback phase in Algorithm~\ref{alg:latent-ml-vl} is modified to compute an eligibility trace from the regularized learning signal $\tilde{\ell}$ as
\begin{align*}
\ell_t = \kappa \ell_{t-1} + (1-\kappa) \bigg( \sum_{i \in \set{X}} \log p(x_{i,t} | u_{i,t}) - \alpha \bigg( \sum_{i \in \set{H}} h_{i,t} \log \frac{\sigma(u_{i,t})}{r} + (1-h_{i,t}) \log \frac{1-\sigma(u_{i,t})}{1-r} \bigg)  \bigg).
\end{align*}
We use a regularization coefficient $\alpha = 1$ and a desired spiking rate $r = 0.1$ for this task. 

For time encoding in Fig.~\ref{fig:prediction_rate_time}, we adopt $N_\textX$ number of truncated Gaussian receptive fields \cite{bohte2002unsupervised}. Considering the value $a_l$ smaller than $0.1$ as silent signal, Gaussian receptive fields are truncated within range $[0.1,1]$, which is discretized into $N_\textX$ uniform regions. Each region is assigned to a Gaussian receptive field, in the sense that the receptive field is chosen to have a mean at a center of the corresponding region and a variance of $1.0$, and then is normalized within the range $[0,\Delta T]$.
